# Supplementary material for: FastTrackTr:Towards Fast Multi-Object Tracking with Transformers
Source: arXiv:2411.15811 source file (2025-07-30)
Supplement: Supplementary file 1 [file suppl.tex]

\clearpage
\appendix

\section{More discussion on FastTrackTr}
\label{appendix_fasttracktr}

\subsection{Description of calculations}
In this section, we analyze the computational complexity of FastTrackTr and MOTR. The goal is to determine the threshold at which the computational cost of the MOTR exceeds that of our FastTrackTr when the number of queries increases. We focus on the decoder layer, including the self-attention, cross-attention, feed-forward network (FFN), and normalization layers.

\subsubsection{Model Definitions}

\textbf{MOTR (Variable Query Number):} The number of queries increases from $N$ to $N_q = N + \Delta N$, where $\Delta N$ is the additional number of queries. Both the self-attention and subsequent components are affected by this increase.

\textbf{FastTrackTr (Modified Self-Attention):} The self-attention mechanism is altered such that the key and value tensors have dimensions $2N \times C$, while the query tensor remains $N \times C$. Other components retain their original computational complexity.

\subsubsection{Notations}

\begin{itemize}
	\item $N$: Original number of queries.
	\item $\Delta N$: Additional queries in MOTR ($N_q = N + \Delta N$).
	\item $C$: Dimensionality of each query.
	\item $M$: Length of the memory (number of keys/values in cross-attention).
	\item $d_{\text{ff}}$: Dimensionality of the FFN's hidden layer (typically $4C$).
\end{itemize}

\subsubsection{Computational Complexity Analysis}

\textbf{MOTR:}

\begin{enumerate}
	\item \textbf{Self-Attention:}
	\begin{align}
		\mathcal{O}_{\text{SA}_1} &= (N + \Delta N)^2 \cdot C
	\end{align}
	
	\item \textbf{Cross-Attention:}
	\begin{align}
		\mathcal{O}_{\text{CA}_1} &= (N + \Delta N) \cdot M \cdot C
	\end{align}
	
	\item \textbf{Feed-Forward Network (FFN):}
	\begin{align}
		\mathcal{O}_{\text{FFN}_1} &= 2(N + \Delta N) \cdot C \cdot d_{\text{ff}}
	\end{align}
	(Two linear layers with activation in between.)
	
	\item \textbf{Layer Normalization:}
	\begin{align}
		\mathcal{O}_{\text{LN}_1} &= 2(N + \Delta N) \cdot C
	\end{align}
	(Two LayerNorm layers.)
\end{enumerate}

\textbf{Total Complexity of MOTR:}
\begin{align}
	\mathcal{O}_{1} &= (N + \Delta N)^2 \cdot C + (N + \Delta N) \cdot M \cdot C \notag \\
	&\quad + 2(N + \Delta N) \cdot C \cdot d_{\text{ff}} + 2(N + \Delta N) \cdot C
\end{align}

\textbf{FastTrackTr:}

\begin{enumerate}
	\item \textbf{Self-Attention:}
	\begin{align}
		\mathcal{O}_{\text{SA}_2} &= N \cdot (2N) \cdot C = 2N^2 \cdot C
	\end{align}
	
	\item \textbf{Cross-Attention:}
	\begin{align}
		\mathcal{O}_{\text{CA}_2} &= N \cdot M \cdot C
	\end{align}
	
	\item \textbf{Feed-Forward Network (FFN):}
	\begin{align}
		\mathcal{O}_{\text{FFN}_2} &= 2N \cdot C \cdot d_{\text{ff}}
	\end{align}
	
	\item \textbf{Layer Normalization:}
	\begin{align}
		\mathcal{O}_{\text{LN}_2} &= 2N \cdot C
	\end{align}
\end{enumerate}

\textbf{Total Complexity of FastTrackTr:}
\begin{align}
	\mathcal{O}_{2} &= 2N^2 \cdot C + N \cdot M \cdot C + 2N \cdot C \cdot d_{\text{ff}} + 2N \cdot C
\end{align}

\subsubsection{Inequality for Computational Cost Comparison}

To find the threshold $\Delta N$ where $\mathcal{O}_{1} > \mathcal{O}_{2}$, we set up the inequality:
\begin{align}
	& (N + \Delta N)^2 \cdot C + (N + \Delta N) \cdot M \cdot C \notag \\
	&\quad + 2(N + \Delta N) \cdot C \cdot d_{\text{ff}} + 2(N + \Delta N) \cdot C \notag \\
	& > 2N^2 \cdot C + N \cdot M \cdot C + 2N \cdot C \cdot d_{\text{ff}} + 2N \cdot C
\end{align}

Simplifying the inequality by eliminating common terms and dividing both sides by $C$:
\begin{align}
	& (N + \Delta N)^2 - 2N^2 + (N + \Delta N - N) \cdot M \notag \\
	&\quad + 2(N + \Delta N - N) \cdot d_{\text{ff}} + 2(N + \Delta N - N) > 0 \notag \\
	\Rightarrow & (N + \Delta N)^2 - 2N^2 + \Delta N \cdot (M + 2d_{\text{ff}} + 2) > 0
\end{align}

Expanding the square term:
\begin{align}
	N^2 + 2N\Delta N + (\Delta N)^2 - 2N^2 \notag \\
	+ \Delta N \cdot (M + 2d_{\text{ff}} + 2) > 0
\end{align}

Combining like terms:
\begin{align}
	- N^2 + 2N\Delta N + (\Delta N)^2 \notag \\
	+ \Delta N \cdot (M + 2d_{\text{ff}} + 2) > 0
\end{align}

Simplifying:
\begin{align}
	- N^2 + \Delta N \left(2N + \Delta N + M + 2d_{\text{ff}} + 2\right) > 0
\end{align}

\subsubsection{Determining the Threshold \texorpdfstring{$\Delta N$}{ΔN}}

To find the minimum $\Delta N$ satisfying the inequality, we proceed as follows.

\begin{align}
	- N^2 + \Delta N \left(2N + \Delta N + M + 2d_{\text{ff}} + 2\right) > 0
\end{align}

\subsubsection{Final Solution with Specific Numerical Values}

Assuming typical values for a Deformable DETR decoder layer:

\begin{itemize}
	\item Number of original queries: $N = 300$
	\item Memory length: $M = 8400$
	\item Query dimensionality: $C = 256$
	\item FFN hidden dimension: $d_{\text{ff}} = 4C = 1024$
\end{itemize}

Substituting the numerical values:
\begin{align}
	- (300)^2 + \Delta N \Big(2 \times 300 + \Delta N + 8400 \notag \\
	+ 2 \times 1024 + 2\Big) > 0
\end{align}

Computing constants:
\begin{align}
	-90,000 + \Delta N \left(600 + \Delta N + 8400 + 2048 + 2\right) > 0
\end{align}

Simplifying the expression inside the parentheses:
\begin{align}
	-90,000 + \Delta N \left(\Delta N + 11,050\right) > 0
\end{align}

Forming a quadratic inequality:
\begin{align}
	(\Delta N)^2 + 11,050 \Delta N - 90,000 > 0
\end{align}

Solving the quadratic equation:
\begin{align}
	(\Delta N)^2 + 11,050 \Delta N - 90,000 = 0
\end{align}

Using the quadratic formula:
\begin{align}
	\Delta N = \frac{ -11,050 \pm \sqrt{(11,050)^2 - 4 \times 1 \times (-90,000)} }{ 2 }
\end{align}

Calculating the discriminant:
\begin{align}
	D &= (11,050)^2 + 360,000 \notag \\
	&= 122,102,500 + 360,000 = 122,462,500
\end{align}

Finding the square root:
\begin{align}
	\sqrt{D} \approx 11,062.83
\end{align}

Determining the positive root:
\begin{align}
	\Delta N = \frac{ -11,050 + 11,062.83 }{ 2 } \approx \frac{12.83}{2} \approx 6.415
\end{align}

The computational cost of MOTR exceeds that of FastTrackTr when the number of additional queries satisfies $\Delta N \geq 7$. This indicates that increasing the number of queries by at least seven will result in higher computational complexity for MOTR compared to FastTrackTr, considering all components of the decoder layer.

In summary, the computational load of FastTrackTr is generally lower than that of MOTR, except in scenarios where there are very few objects to track; in those cases, the theoretical computation may be slightly higher for FastTrackTr. Otherwise, FastTrackTr consistently requires less computational effort. Additionally, in practical applications, MOTR tends to be significantly slower due to memory constraints. For a detailed analysis, please refer to Section. \ref{MOTR_Speed}.

\subsection{Why Circle Loss}

The empirical superiority of Circle Loss in Table~\ref{loss_ablation} originates from fundamental alignment between its optimization dynamics and the architectural characteristics of DETR-based tracking.  In this section ,We provide a multi-perspective analysis.

In DETR, object queries are learnable vectors representing potential object instances with joint spatial and semantic information. They interact with image features via cross-attention, forming vectors containing spatial coordinates and semantic features. These vectors are mapped to detection results like bounding box coordinates and class probabilities through detection heads. Our work extends this by adding an ID embedding head to the existing classification and regression branches. This head, implemented via a fully connected layer, maps object queries to a trackable feature space for discriminative features for target association. Moreover, we adopt a joint optimization strategy during training to balance detection accuracy and identity representation effectiveness. This ensures the additional module doesn't compromise detection performance, maintaining a robust model for both detection and tracking.

Let $\mathbf{q}_t^i \in \mathbb{R}^D$ denote the $i$-th object query at frame $t$, which encodes both spatial coordinates $(x,y,w,h)$ and appearance features through transformer attention. The gradient flow for embedding learning can be expressed as:

\begin{equation}
	\frac{\partial \mathcal{L}}{\partial \mathbf{q}_t^i} = \sum_{j\in\mathcal{P}} \frac{\partial \mathcal{L}}{\partial s_p^j} \frac{\partial s_p^j}{\partial \mathbf{q}_t^i} + \sum_{k\in\mathcal{N}} \frac{\partial \mathcal{L}}{\partial s_n^k} \frac{\partial s_n^k}{\partial \mathbf{q}_t^i}
\end{equation}

For Circle Loss, the gradient magnitudes adaptively scale with sample hardness:
\begin{equation}
	\left|\frac{\partial \mathcal{L}_{\text{circle}}}{\partial s_p}\right| = \gamma\alpha_p, \quad \left|\frac{\partial \mathcal{L}_{\text{circle}}}{\partial s_n}\right| = \gamma\alpha_n
\end{equation}

This creates \textit{dynamic gradient reweighting} where:
\begin{itemize}
	\item Queries with ambiguous matches ($s_p \approx 1-m$) receive stronger positive gradients
	\item Challenging negatives ($s_n \approx m$) obtain amplified negative gradients
\end{itemize}

In contrast, Triplet Loss applies constant margin enforcement regardless of prediction confidence, causing two issues:
\begin{itemize}
	\item Over-penalization of well-separated samples (wasted capacity)
	\item Insufficient focus on borderline cases (critical for MOT)
\end{itemize}

To be more specific, we can compare the visual representation of query embedding space with further analysis. Let $\mathcal{Q} \subset \mathbb{R}^D$ be the query embedding space:

\begin{itemize}
	\item \textbf{Triplet Loss}: Enforces fixed Euclidean margin $\alpha$ between positive/negative pairs
	\begin{equation}
		\|\mathbf{q}_t^i - \mathbf{q}_{t+1}^j\|_2^2 + \alpha < \|\mathbf{q}_t^i - \mathbf{q}_{t+1}^k\|_2^2
	\end{equation}
	
	\item \textbf{Circle Loss}: Establishes adaptive angular margins in cosine space
	\begin{equation}
		\cos\theta_p > \cos\theta_n + m
	\end{equation}
\end{itemize}

The angular formulation better aligns with DETR's dot-product attention mechanism, creating geometrically compatible gradients that reinforce the inherent transformer operations.

%Our frame-sequential computation creates temporal chains of gradient propagation:
%
%\begin{equation}
%	\mathbf{q}_{t+1}^j = \text{Attn}(\mathbf{q}_t^j, \mathbf{X}_{t+1}) + \mathbf{q}_t^j
%\end{equation}
%
%Circle Loss enhances temporal stability through:
%\begin{itemize}
%	\item \textbf{Forgetting Resistance}: Hard positive samples maintain strong gradient signals across frames
%	\item \textbf{Drift Prevention}: Adaptive margin adjustment counters gradual feature displacement
%\end{itemize}

\subsubsection{Discussion on other losses}
In past loss functions and newer Transformer-based tracking framework losses, several issues arise in our model context. MOTIP and PuTR's loss functions, centered on matching and ID prediction, are unsuitable for query - based approaches. JDE's original loss faces dimensionality and optimization challenges in training. Let's delve into these issues:

MOTIP's ID dictionary $\mathcal{D} \in \mathbb{R}^{M\times D}$ with static entries conflicts with DETR's dynamic query binding:

\begin{equation}
	\mathcal{L}_{\text{MOTIP}} = \sum_{i=1}^{N_q} \|\mathbf{q}_t^i - \mathcal{D}[y_t^i]\|_2^2
\end{equation}

This formulation fails when $y_t^i$ changes across frames (common in occlusion recovery), causing dictionary index collisions. Our method avoids this through query-specific embedding learning without ID-to-vector locking.

PuTR prioritizes motion coherence through:

\begin{equation}
	\mathcal{S}_{\text{PuTR}}(i,j) = \lambda_{\text{app}}s(f_i,f_j) + \lambda_{\text{mot}}\mathcal{N}(\Delta\mathbf{b}_{ij}|\mu,\Sigma)
\end{equation}

The motion term $\mathcal{N}(\Delta\mathbf{b}_{ij}|\mu,\Sigma)$ conflicts with our queries' spatial priors already encoding box coordinates $\mathbf{b}_i$. This creates contradictory optimization signals:

\begin{equation}
	\frac{\partial \mathcal{S}_{\text{PuTR}}}{\partial \mathbf{q}_i} = \lambda_{\text{app}}\frac{\partial s}{\partial \mathbf{q}_i} + \lambda_{\text{mot}}\frac{\partial \mathcal{N}}{\partial \mathbf{b}_i}\frac{\partial \mathbf{b}_i}{\partial \mathbf{q}_i}
\end{equation}

The second term disrupts the coordinated spatial-semantic encoding learned by the transformer.

JDE's ID prediction as classification:

\begin{equation}
	\mathcal{L}_{\text{JDE}} = -\sum_{i=1}^{N_q} y_t^i \log p(\hat{y}_t^i)
\end{equation}

This requires fixing the number of identities $|\mathcal{Y}|$, fundamentally incompatible with our video-agnostic design where $\mathcal{Y}$ varies across sequences. Our approach's pairwise metric learning eliminates this constraint.

\subsection{Temporal-Consistent Learning Paradigm}
\label{sec:temporal_training}

The adoption of temporal slice training in FastTrackTr stems from its intrinsic alignment with the temporal modeling characteristics of our encoder-decoder architecture. Unlike conventional frame-wise training that treats video sequences as independent snapshots, our approach enforces temporal coherence through two synergistic mechanisms. First, the temporal adjacency constraint in the ReID loss induces gradient flows that propagate identity information across consecutive frames. Specifically, the Markovian gradient equation:

\begin{equation}
	\nabla_{\mathbf{q}_t^i}\mathcal{L}_{\text{reid}} = \sum_{\delta=1}^{\Delta t} \frac{\partial \mathcal{L}(t,t+\delta)}{\partial \mathbf{q}_t^i} 
\end{equation} creates cumulative learning signals that strengthen the encoder's capability to extract temporally stable features. This gradient accumulation effect is particularly crucial for the historical encoder's masking mechanism, as it teaches the model to distinguish between transient occlusions and permanent identity changes through progressive exposure to local temporal windows.

The decoder's historical cross-attention mechanism benefits from this training paradigm through implicit temporal regularization. By processing concatenated historical and current queries in sliding windows, the model learns to establish soft associations between object representations across frames. This process is stabilized by the temporal gradient structure, which prevents attention weights from overfitting to short-term appearance variations. The synergy becomes evident during occlusions: while the encoder maintains stable identity embeddings through temporal averaging of gradients, the decoder learns to bridge occlusion gaps by attending to reliable historical queries.

Furthermore, the slice-wise training acts as a regularizer for the dynamic masking strategy in the historical encoder. As the model processes sequences in temporal chunks, it gradually learns to adjust the mask generation parameters based on local context reliability. This contrasts with full-sequence training where global error propagation could overwhelm the delicate balance between historical information retention and noise suppression. The temporal windowing also enables curriculum-like learning - starting with short-term dependencies and progressively handling longer temporal relationships as training proceeds.

The effectiveness of this design is rooted in the complementary roles of encoder and decoder in temporal modeling. The encoder's masked self-attention operates as a temporal filter, suppressing inconsistent features through gradient-driven parameter updates. Meanwhile, the decoder's cross-attention serves as a temporal integrator, combining filtered historical states with current observations. The temporal training paradigm ensures both components evolve in concert, creating a positive feedback loop where improved temporal filtering enables better integration, which in turn provides cleaner signals for subsequent filtering.

\subsection{Possibilities of End-to-end}
We originally developed FastTrackTr with the goal of proposing a real-time, end-to-end multi-object tracking model. However, we observed that eliminating one decoder and directly applying MOTIP's ID loss resulted in significant challenges in model convergence. Upon further analysis, we determined that although MOTIP's ID loss appears similar to the appearance loss used in the previous JDT models, they fundamentally differ.

\begin{figure}[t]
	\begin{center}
		\includegraphics[width=1\linewidth]{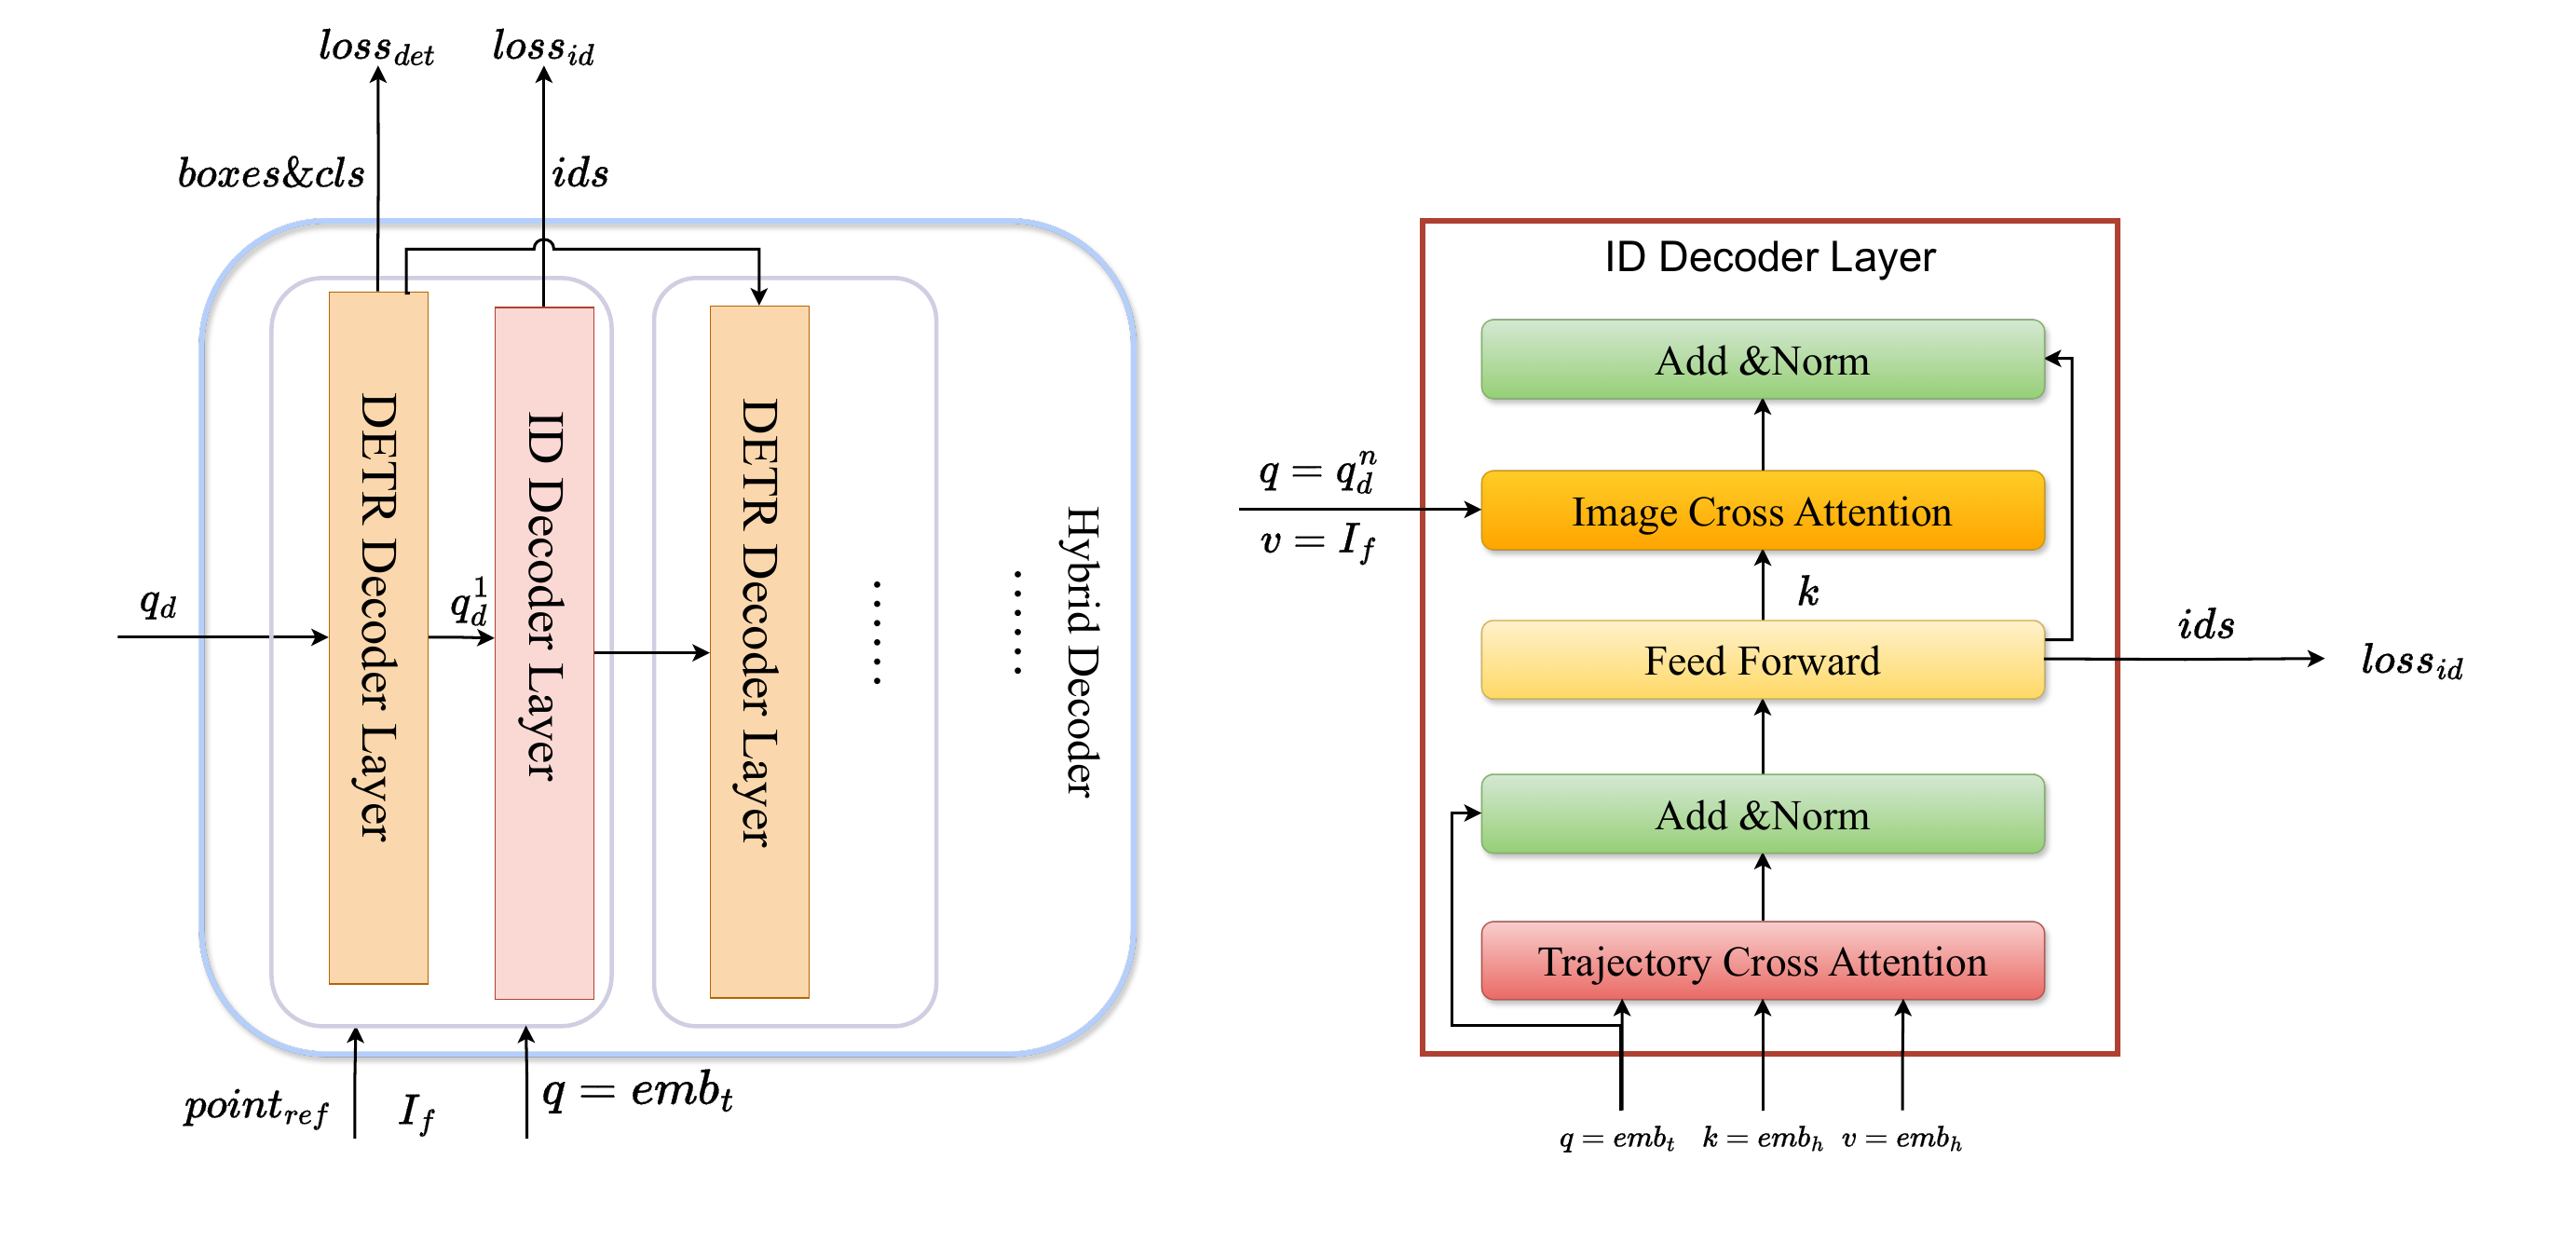}
	\end{center}
	\caption{The proposed architecture features a hybrid decoder capable of facilitating end-to-end rapid tracking, which currently consists of six layers. There are two distinct types of layers within this decoder: the standard DETR layers, which are used to output detection results, and the ID decoder layers, which are dedicated to producing tracking outcomes. These layers are arranged alternately, with each type comprising three layers. This design aims to effectively merge detection and tracking functionalities within a single streamlined framework.}
	\label{end2end}
\end{figure}

For models like JDE \cite{wang2020towards}, the focus is on the similarity of object appearances, which does not incorporate specific object trajectories. In contrast, the ID decoder in MOTIP primarily handles trajectory information, with image data serving only as a supplementary element. The function and training method of this decoder might be similar to the entire PuTR model. Although our FastTrackTr attempts to integrate some temporal information by passing queries from one frame to the next, these queries predominantly contain image features. Under such conditions, supervising motion trajectories directly using MOTIP's method becomes less effective, leading to poor or nearly impossible model convergence.

Following this analysis, we attempted to incorporate more historical information into the decoder. Our preliminary design introduces an identity-specific decoder layer into the traditional DETR architecture, as illustrated in Figure.\ref{end2end}. These layers enhance alignment between current frame detections and corresponding identity features through a two-step attention mechanism, and link current detections with historical trajectories by emphasizing temporal consistency. The ID decoder layers are interlaced with standard DETR layers, initially comprising six layers in total.

The trajectory attention within the ID decoder layers can be formally described as follows:

\begin{align} 
	\begin{aligned}
		& Q_{ID} = emb_t, \quad K_{ID} = V_{ID} = emb_h  \\
		& A_{ID} = \operatorname{Softmax}\left(\frac{Q_{ID} K_{ID}}{\sqrt{C}}\right) \\
		&\quad q^{\prime}_{ID} = A_T V_T 
	\end{aligned}
\end{align}
where $emb_t$ and the input id decoder in MOTIP are the same. Its main components are the output of the previous decoder layer and the id encoding. $emb_h$ is the historical encoding. Finally, the $q^{\prime}_{ID} \in \mathbb{R}^{2\times N \times C}$ will be reduced in dimension and fused through a conv layer and an FFN layer in the feedforward network. 

The id loss used after the feedforward neural network and the id head is the id loss of MOTIP, which is shown below:

\begin{align}
	\begin{aligned}
		& \mathcal{L}_{i d}=\frac{-\sum_{t=2}^{T+1} \sum_{m=1}^{M_t} \sum_{k=1}^{K+1} y_m^k \log \left(p_m^k\right)}{\sum_{t=2}^{T+1} M_t}, \\
		& y_m^k= \begin{cases}1 & \mathrm{gt}_{id} \text { of } m^{t h} \text { object is } k, \\
			0 & \text { else },\end{cases}
	\end{aligned}
\end{align}

where $T+1$ denotes the number of frames in a training clip, while there are $M_t$ ground-truth objects in the $t$-th frame. $y_m^k$ is an indicator function according to the identity ground truth of each object, as shown in Eq.(\ref{end2endqe}) . In practice, we simultaneously train object detector and ID predictor in an end-to-end strategy. Therefore, we leverage an overall loss function $\mathcal{L}$ to supervise these two parts:
\begin{align}
	\label{end2endqe}
	\mathcal{L}=\lambda_{\text {det}} \mathcal{L}_{\text {det}}+\lambda_{\text {id }} \mathcal{L}_{\text {id }}
\end{align}

Due to time constraints and the incomplete state of the model, we have conducted only one epoch of training on the DanceTrack dataset to observe whether the loss converges. After this single epoch, when employing the MOTIP process during inference, the HOTA score was approximately 16.7. This result preliminarily confirms that the model is broadly effective, with further fine-tuning required to optimize its performance.

\subsection{Improvements of the JDE association module}
We believe that one of the reasons why JDT-type models have gradually been abandoned in recent years is that the commonly used JDE \cite{wang2020towards} association module has become somewhat outdated. This has led to JDT models underperforming compared to some of the more recent models. To better demonstrate the superiority of our approach, we made some minor adjustments to the JDE association method to improve its tracking performance.

Our improvements mainly focus on two aspects:
\begin{itemize}
	\item [1)] In the JDE association module, we associate only high-confidence detection boxes, ignoring those with lower confidence scores. By incorporating ByteTrack’s \cite{zhangByteTrackMultiobjectTracking2022} bi-stage matching mechanism, we temporarily retain these low-confidence detection boxes as candidate targets. After matching the high-confidence targets, we perform a second round of matching using the high-confidence targets, which enhances tracking performance to some extent.
	\item [2)] We also made some adjustments to the association strategy. In JDE, the first association is typically based on ID features, followed by a second association using historical trajectories. In our approach, similar to many other trackers, we include historical trajectories in the first round of association. Specifically, the cost matrix $C$ is the weighted sum of the appearance cost $A_a$ and the motion cost $A_m$, as follows:
\end{itemize}
\begin{figure}[t]
	\begin{center}
		\includegraphics[width=1\columnwidth]{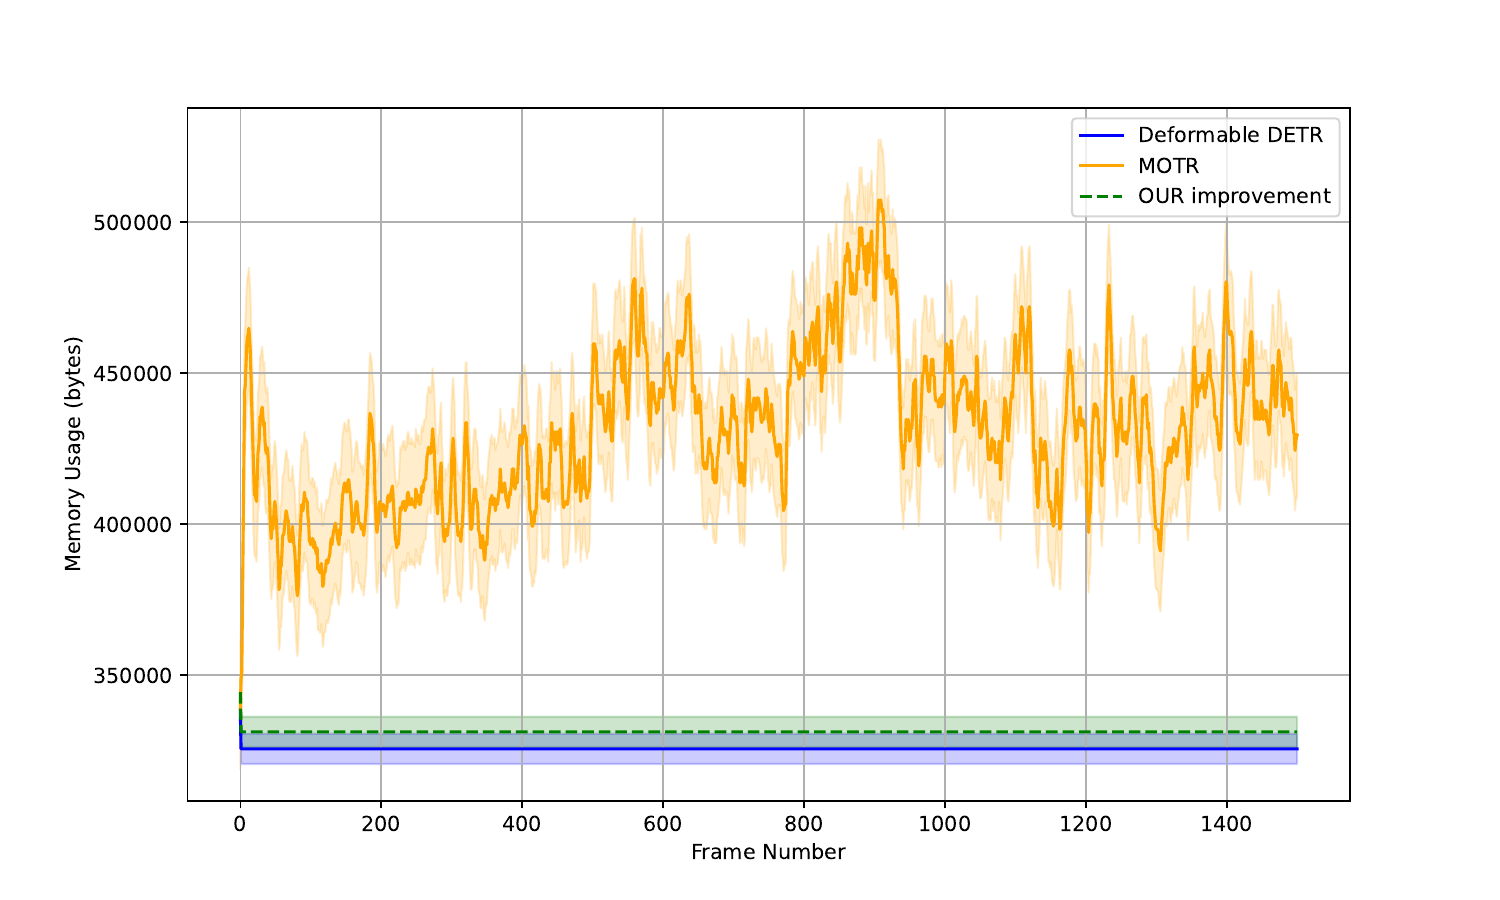}
	\end{center}
	\caption{The changes in GPU memory consumption after the decoder for the MOTR, Deformable DETR, and our improved model in MOT17-03.}
	\label{memory}
\end{figure}

\begin{figure}[t]
	\begin{center}
		\includegraphics[width=1\linewidth]{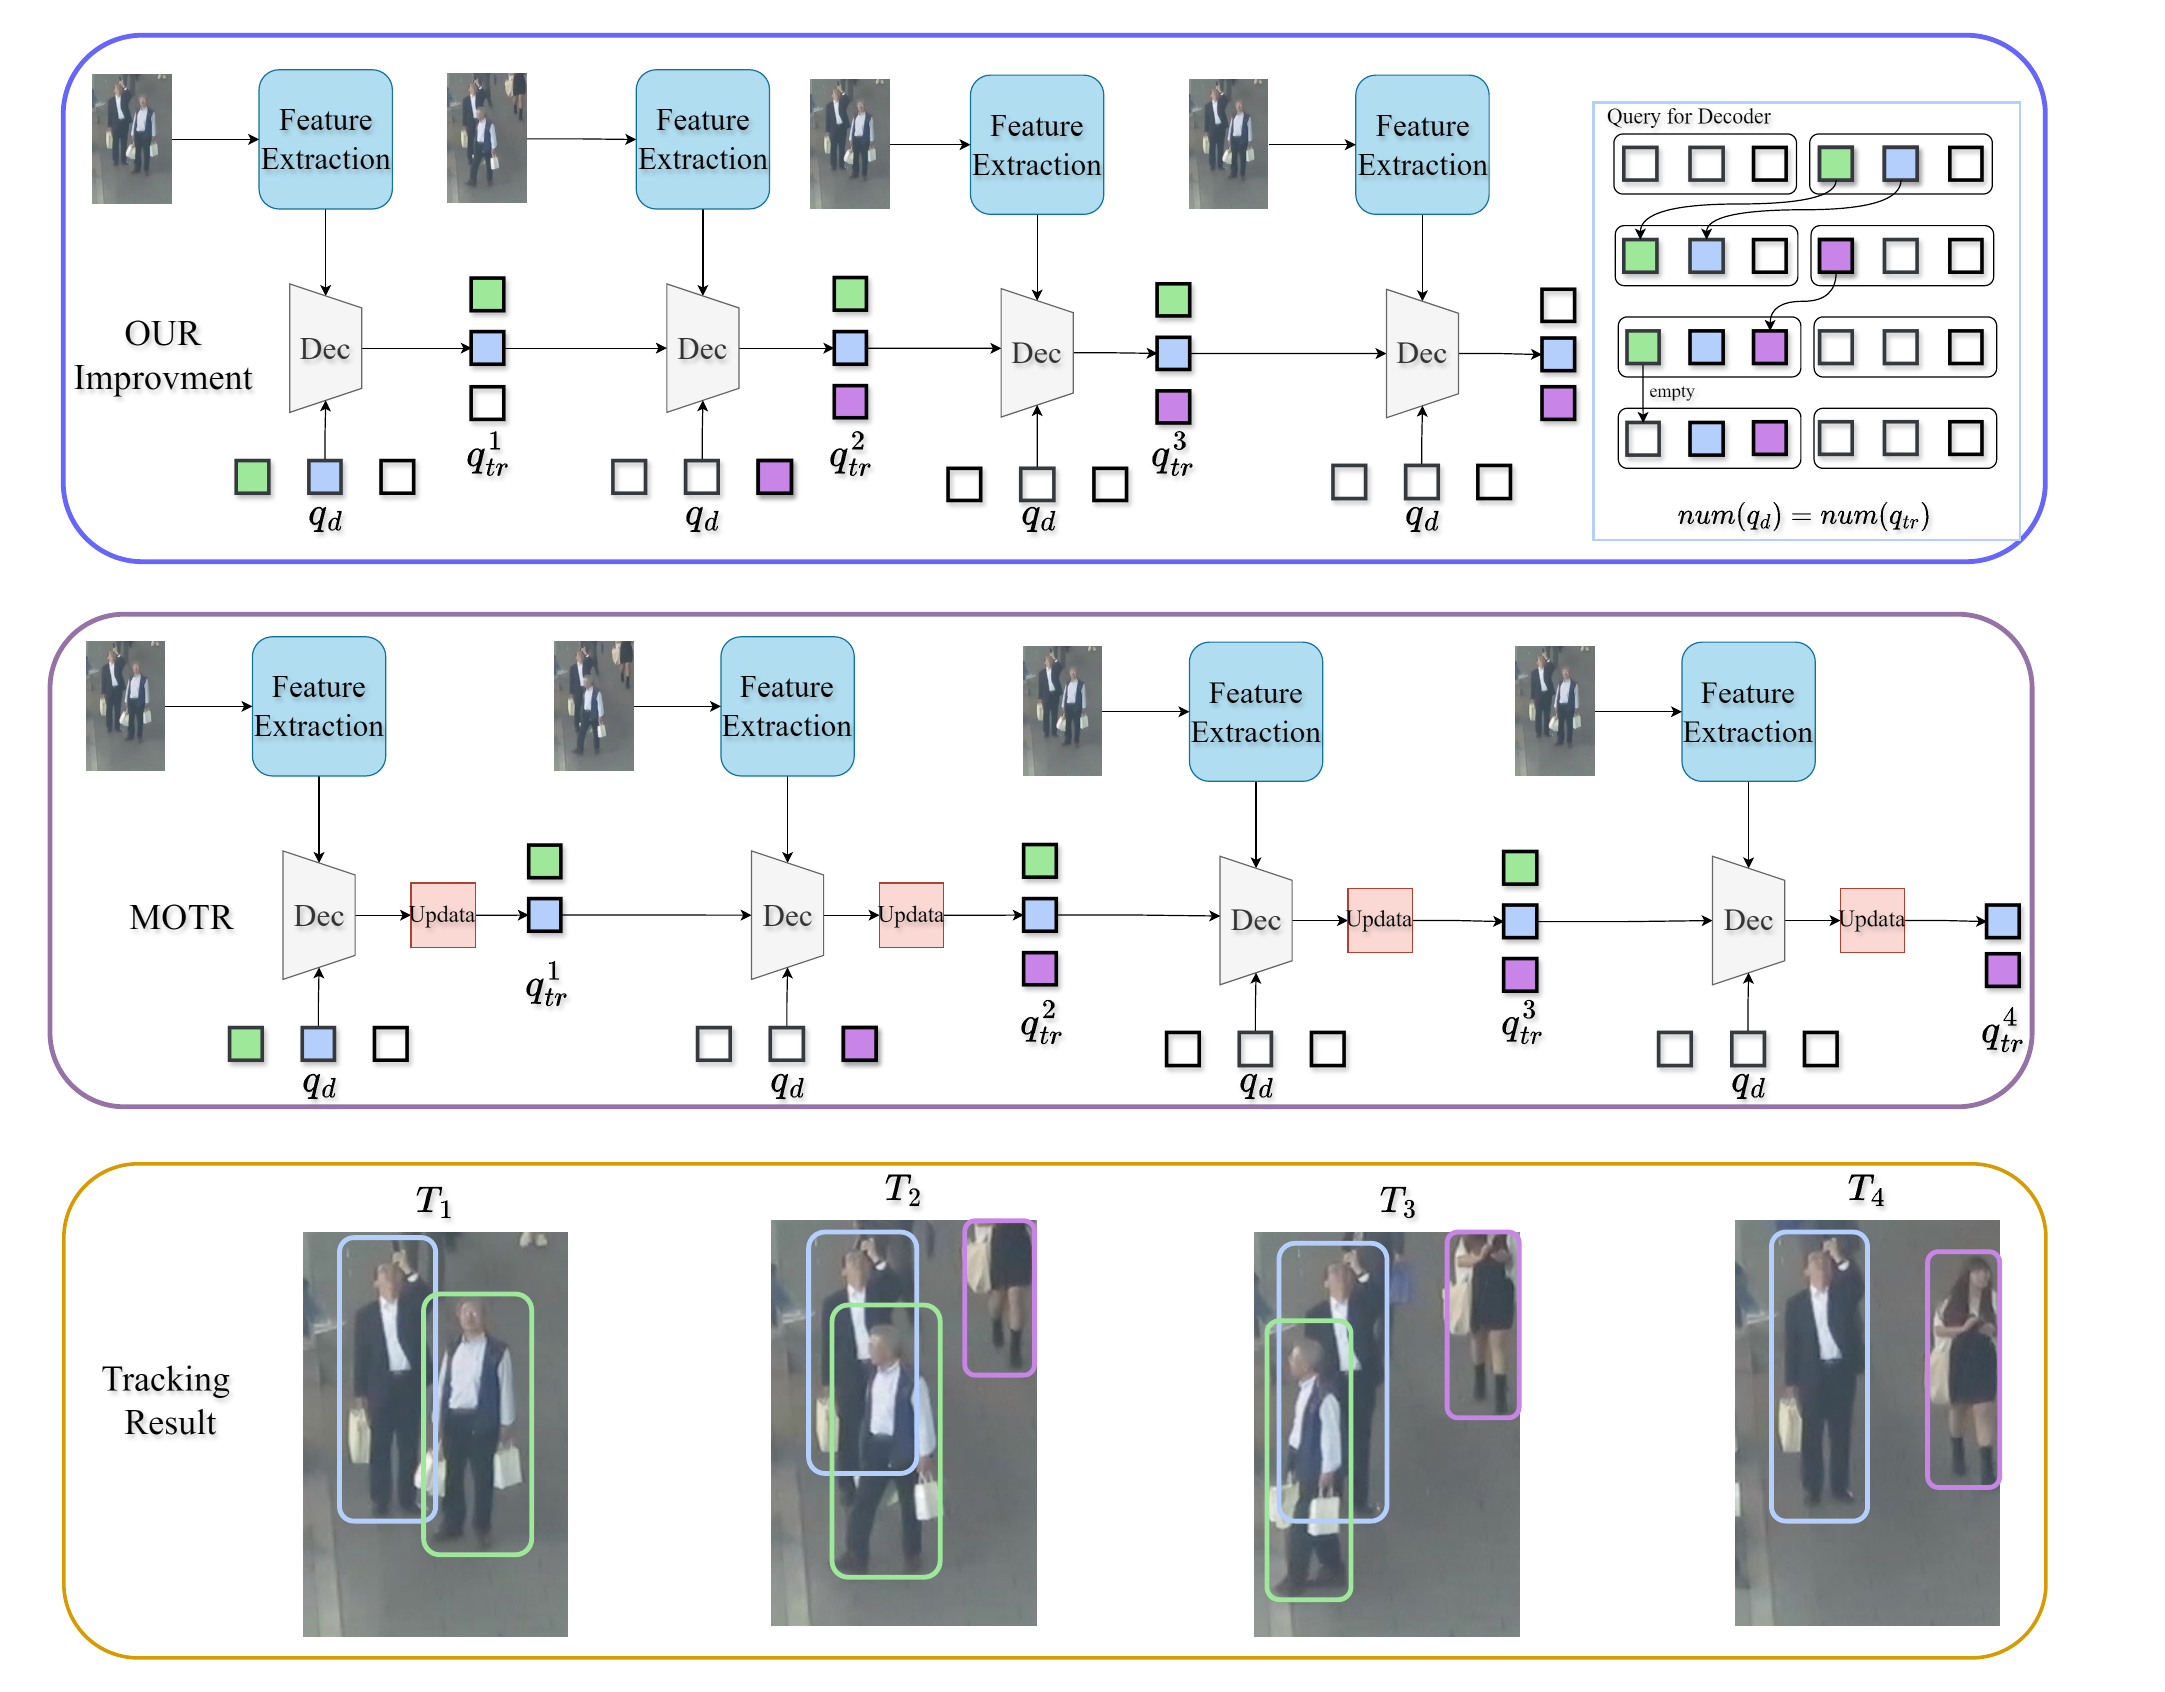}
	\end{center}
	\caption{A simple MOTR and our improved tracking process diagram. The number of queries for MOTR will change, but after our improvement, it remains unchanged.}
	\label{MOTR}
\end{figure}

\begin{align}
	C=\lambda A_a+(1-\lambda) A_m
\end{align}

where the weight factor $\lambda$ is set to  0.99 , as in \cite{maggiolinoDeepOCSORTMultiPedestrian2023,yang2024hybrid} . 

\begin{table}
	\centering
	\label{association}
	\caption{Ablation Study of association module on the DanceTrack validation set.}
	\resizebox{!}{!}{
		\begin{tabular}{c|c|cccc}\hline
			Byte	& Cost  & HOTA & DetA   & AssA &IDF1 \\ \hline
			&    &  51.5  & 72.4& 37.5 & 51.4\\
			$\checkmark$ & &  53.4  & 74.3& 39.7 & 53.1 \\
			& $\checkmark$ &  52.4  & 73.1& 38.3 & 52.6 \\
			$\checkmark$ & $\checkmark$ &    54.1  & 75.6& 40.0 & 54.7 \\
			
			\hline
		\end{tabular}
	}
\end{table}

\subsection{More Implementation Details}

By default, on DanceTrack \cite{sunDanceTrackMultiObjectTracking2022}, we train FastTrackTr for 27 epochs on the training set, dropping the learning rate by a factor of 10 at the 14th and 18th epochs. On SportsMOT \cite{cui2023sportsmot}, we train our model for 27 epochs on the training set, with the learning rate dropped at the 14th and 18th epochs. On MOT17 \cite{milanMOT16BenchmarkMultiObject2016}, we train the model on this combined training set for 80 epochs, with the learning rate dropped at the 45th and 55th epochs.

For the additional use of the CrowdHuman dataset on DanceTrack and MOT17, our usage method follows the same approach as MOTIP. Interested readers can refer to the original work for further details.

\subsection{Details about TensorRT acceleration and the running speed of our method on edge devices}

As previously noted, MOTIP presents significant challenges for TensorRT acceleration due to dynamic data flow characteristics. While this essentially constitutes an engineering optimization issue with limited academic novelty - hence our prior omission of detailed discussion - we hereby provide technical clarification.

The dynamic data patterns in both MOTIP and MOTR architectures do not originate from input dimension variability, but rather emerge during model operation through internal state transitions. Specifically, in MOTIP, dynamic states manifest in the posterior identity prediction network, while in MOTR, dynamic computation occurs within the DETR decoder module.

This architectural implementation creates non-trivial engineering obstacles when converting models to TensorRT, as existing conversion tools (v10.8.0.43 in our tests) primarily support dynamic input dimensions rather than mid-network dynamic state transitions. The hybrid static-dynamic data flow requires either PyTorch code restructuring with mask operations to enforce static dimensionality or complete network reconstruction using native TensorRT functions with weight remapping. Given the substantial engineering effort required, we deferred these optimization attempts.

Notably, PuTR demonstrates convertible capability through standard toolchains, yet only achieves 80$\%$ acceleration efficiency in our development environment. We hypothesize this performance gap stems from memory scheduling inefficiencies similar to MOTR's limitations, though mitigated by PuTR's lightweight architecture.

Final benchmarking results across MOT frameworks on the edge computing platform (NVIDIA Jetson AGX Orin, TensorRT 10.8.0.43) are systematically presented in Table 11, with detailed latency breakdowns and memory utilization metrics.

\section{How to Improve MOTR inference Speed}
\label{MOTR_Speed}

Although we have demonstrated in the previous sections that our FastTrackTr model generally requires less computation than the MOTR series of models, there remains an issue that puzzles us. Under the same configuration, models such as Deformable-DETR, MOTIP, and our FastTrackTr typically push GPU utilization to around 90$\%$. However, MOTR only reaches about 40$\%$ on the same hardware (e.g., an RTX 4090), which is clearly problematic. 

This led us to speculate whether the issue might be due to the dynamic nature of the query system, which could result in variable memory usage. As shown in Figure \ref{memory}, we compare the memory consumption of the decoder when using fixed queries versus dynamic queries. After further investigation, we found that this is indeed a plausible cause. In cuda, memory is managed through cudaMalloc and cudaFree. These operations incur significant computational overhead. To mitigate this, PyTorch attempts to reuse memory blocks previously allocated via cudaMalloc. When a suitable cached block exists in PyTorch's allocator, it directly serves the request without invoking cudaMalloc, thereby minimizing latency during initial allocation phases. However, MOTR's dynamic data patterns require intermediate tensors of varying sizes throughout runtime. This variability prevents the allocator from leveraging cached blocks of appropriate dimensions, forcing frequent calls to cudaFree to release outdated allocations and subsequent cudaMalloc requests for new memory spaces. Consequently, the allocator repeatedly rebuilds its caching infrastructure through bulk CUDA API operations – an expensive process that introduces substantial latency spikes. This thrashing behavior substantially degrades computational efficiency and hinders full GPU utilization

We experimented with PyTorch’s memory management code, and observed that when the tensor size remains relatively constant, there are significantly fewer memory allocation and release calls. The specific code we tested can be easily found in GitHub, when you search for 'torch mem'(we would like to note that the owner of that link is not associated with the authors of this paper.

% \href{https://github.com/CalvinXKY/BasicCUDA/tree/master/pytorch/torch1.13_mem_rationale}{here} (we would like to note that the owner of this link is not associated with the authors of this paper). PyTorch 2’s memory management, apart from supporting expandable segments, remains consistent with version 1.13.

So how can we address this issue? Modifying PyTorch’s underlying logic directly is quite complex and would likely require intervention from PyTorch’s developers (we are preparing to submit an issue on GitHub or send an email to the maintainers). An alternative approach could be to fix the number of tracking queries in MOTR and use masks to differentiate between empty tracking queries and those that are actively used. This may resolve the issue. As shown in Figure \ref{MOTR}, we trained an updated version of MOTR for one epoch on the DanceTrack dataset and tested the speed and GPU utilization. Due to limitations in funding, equipment, and time, we did not fully train the model to evaluate its performance. However, preliminary results show promise: after one epoch, the HOTA score on the validation set reached 18.5 and fps has increased from 16.5 to 25 with fp32 precision. Note that we have not reduced any network structure at this time. Interested readers are welcome to experiment with this approach themselves. It is relatively straightforward to implement, though we advise against using GPUs with less than 24GB of memory, as this may lead to out-of-memory errors.

Of course, this is just one possible explanation. Other factors may also contribute to the underutilization of GPU resources in MOTR-like models. If any readers have alternative insights, we welcome further discussion and collaboration.

\section{Visualization of FastTrackTr Results}
In this section, we will provide visualization results of our model on different datasets.

\begin{figure*}[t]
	\begin{center}
		\includegraphics[width=1\textwidth]{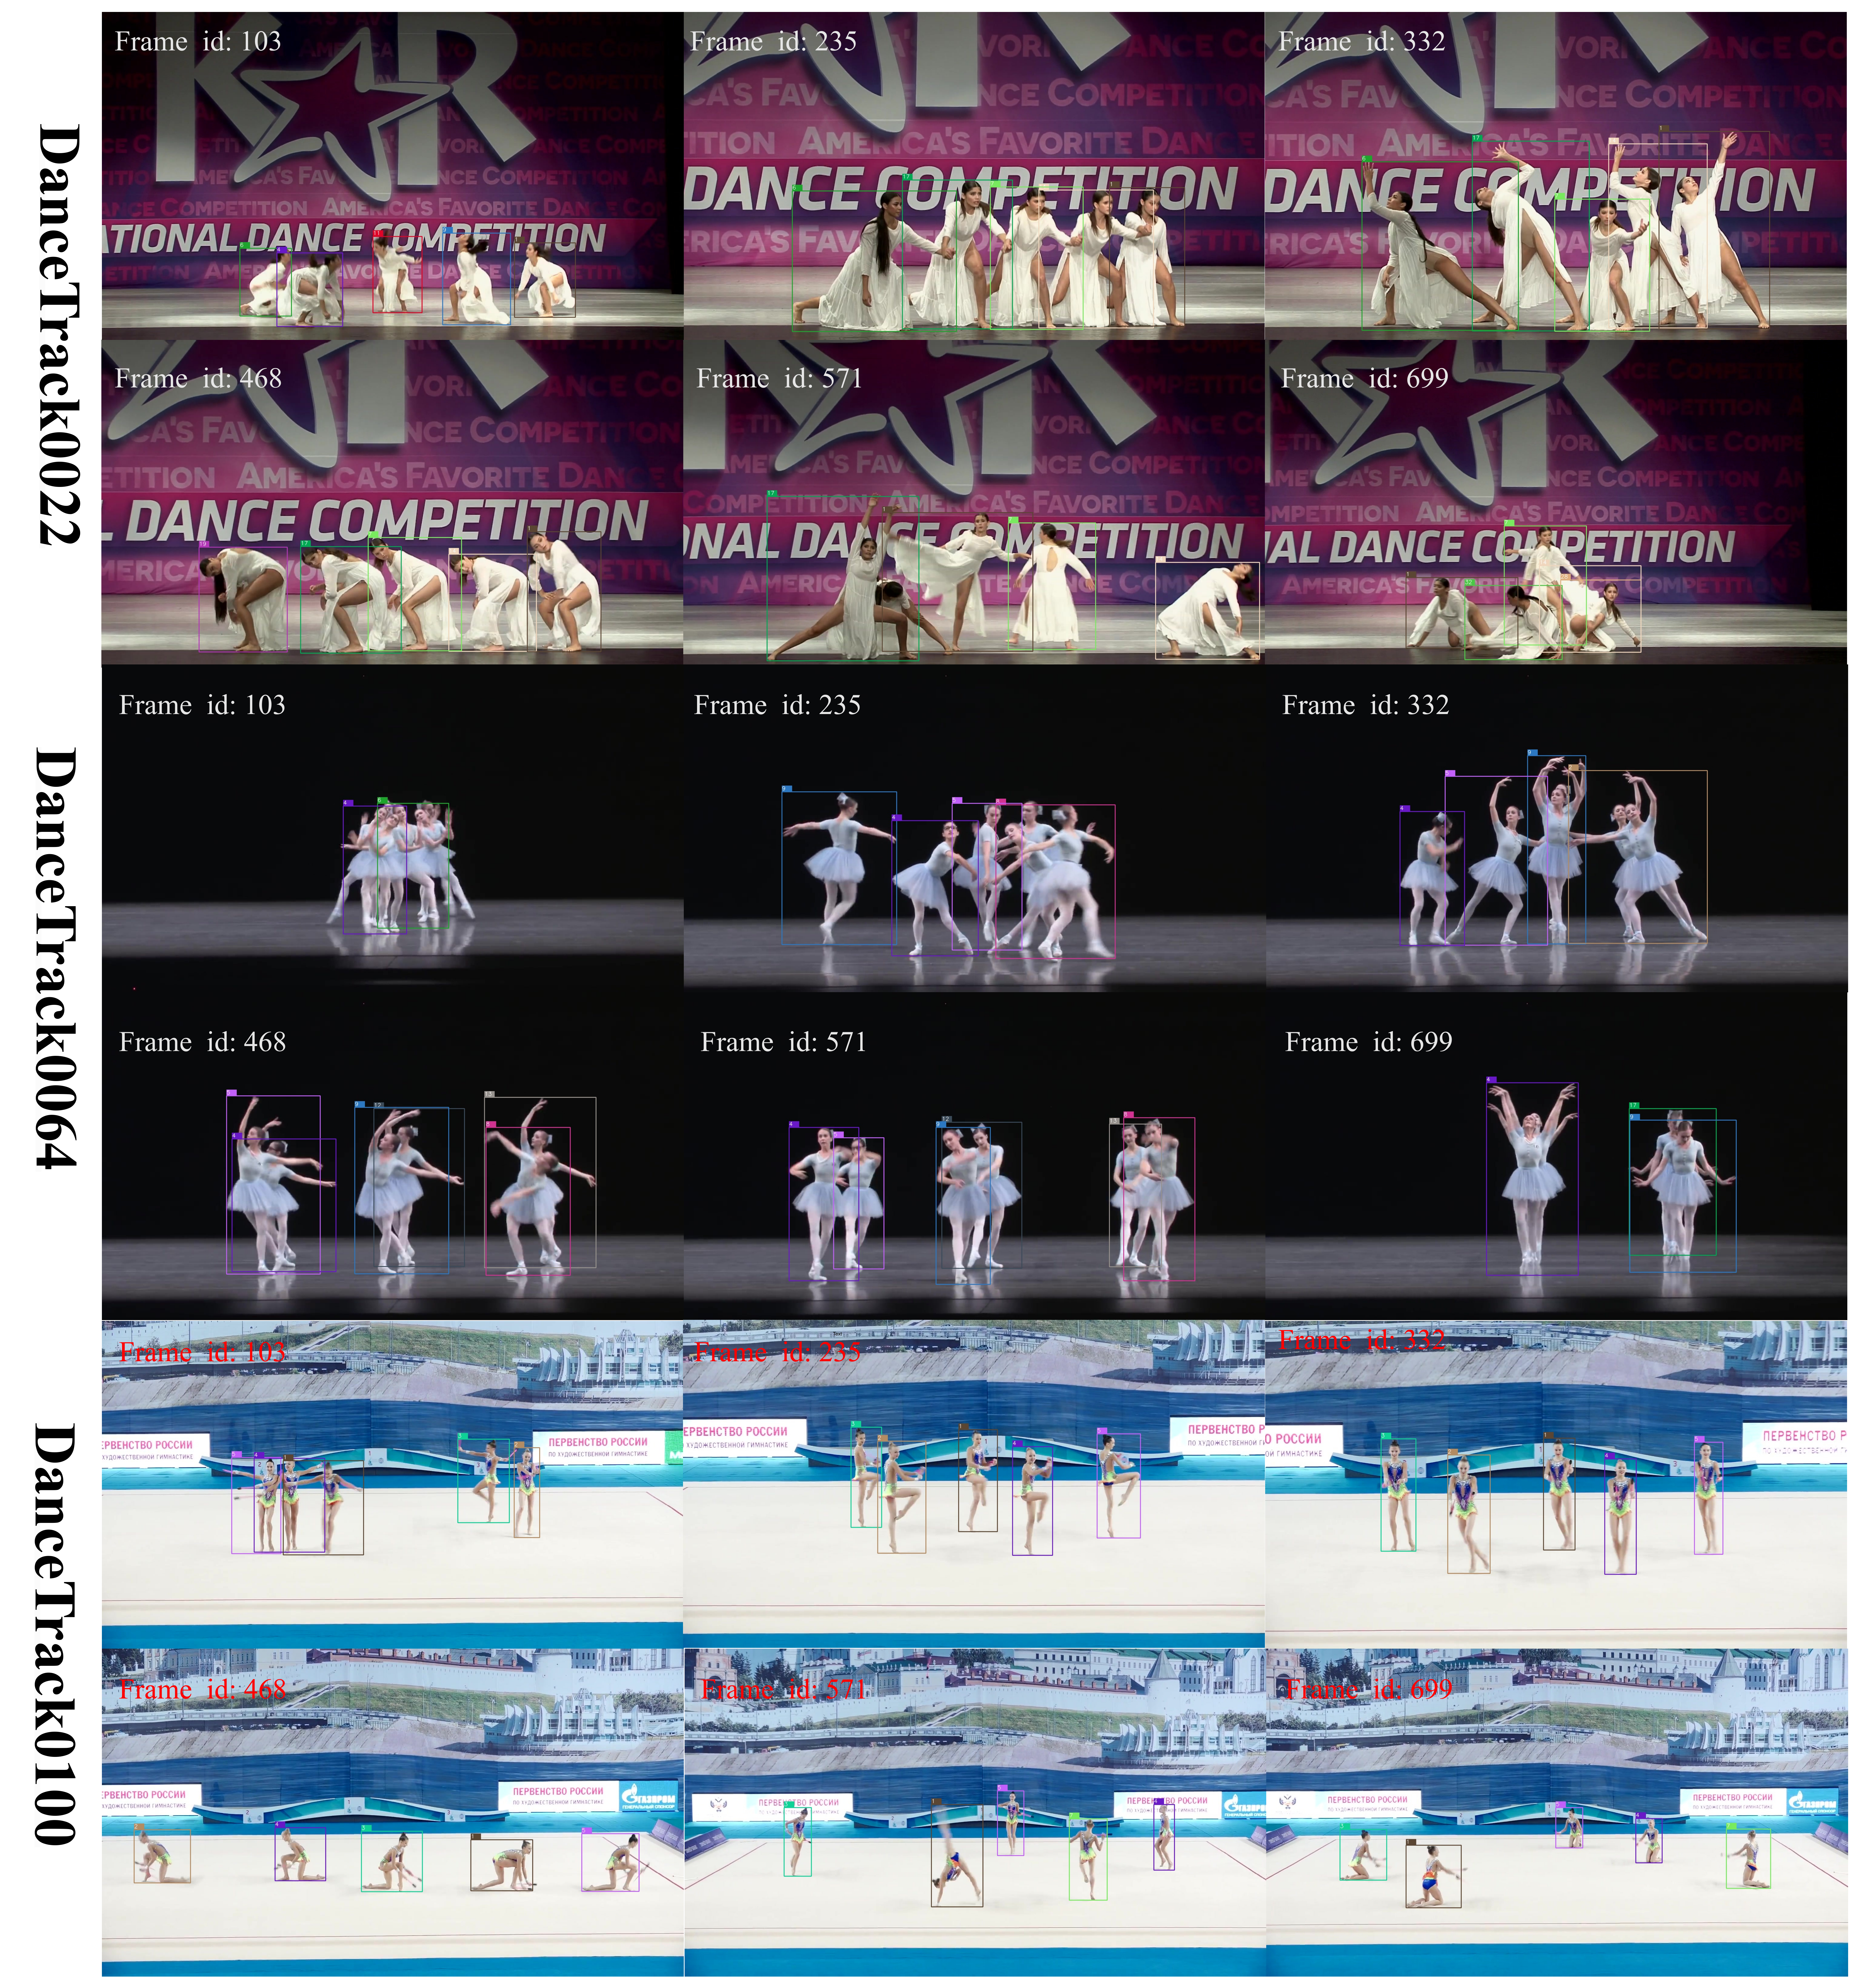}
	\end{center}
	\caption{Our model's visualization results on Dancetrack, where the same color represents the same object.}
	\label{vis_result_dance}
\end{figure*}

\begin{figure*}[t]
	\begin{center}
		\includegraphics[width=1\textwidth]{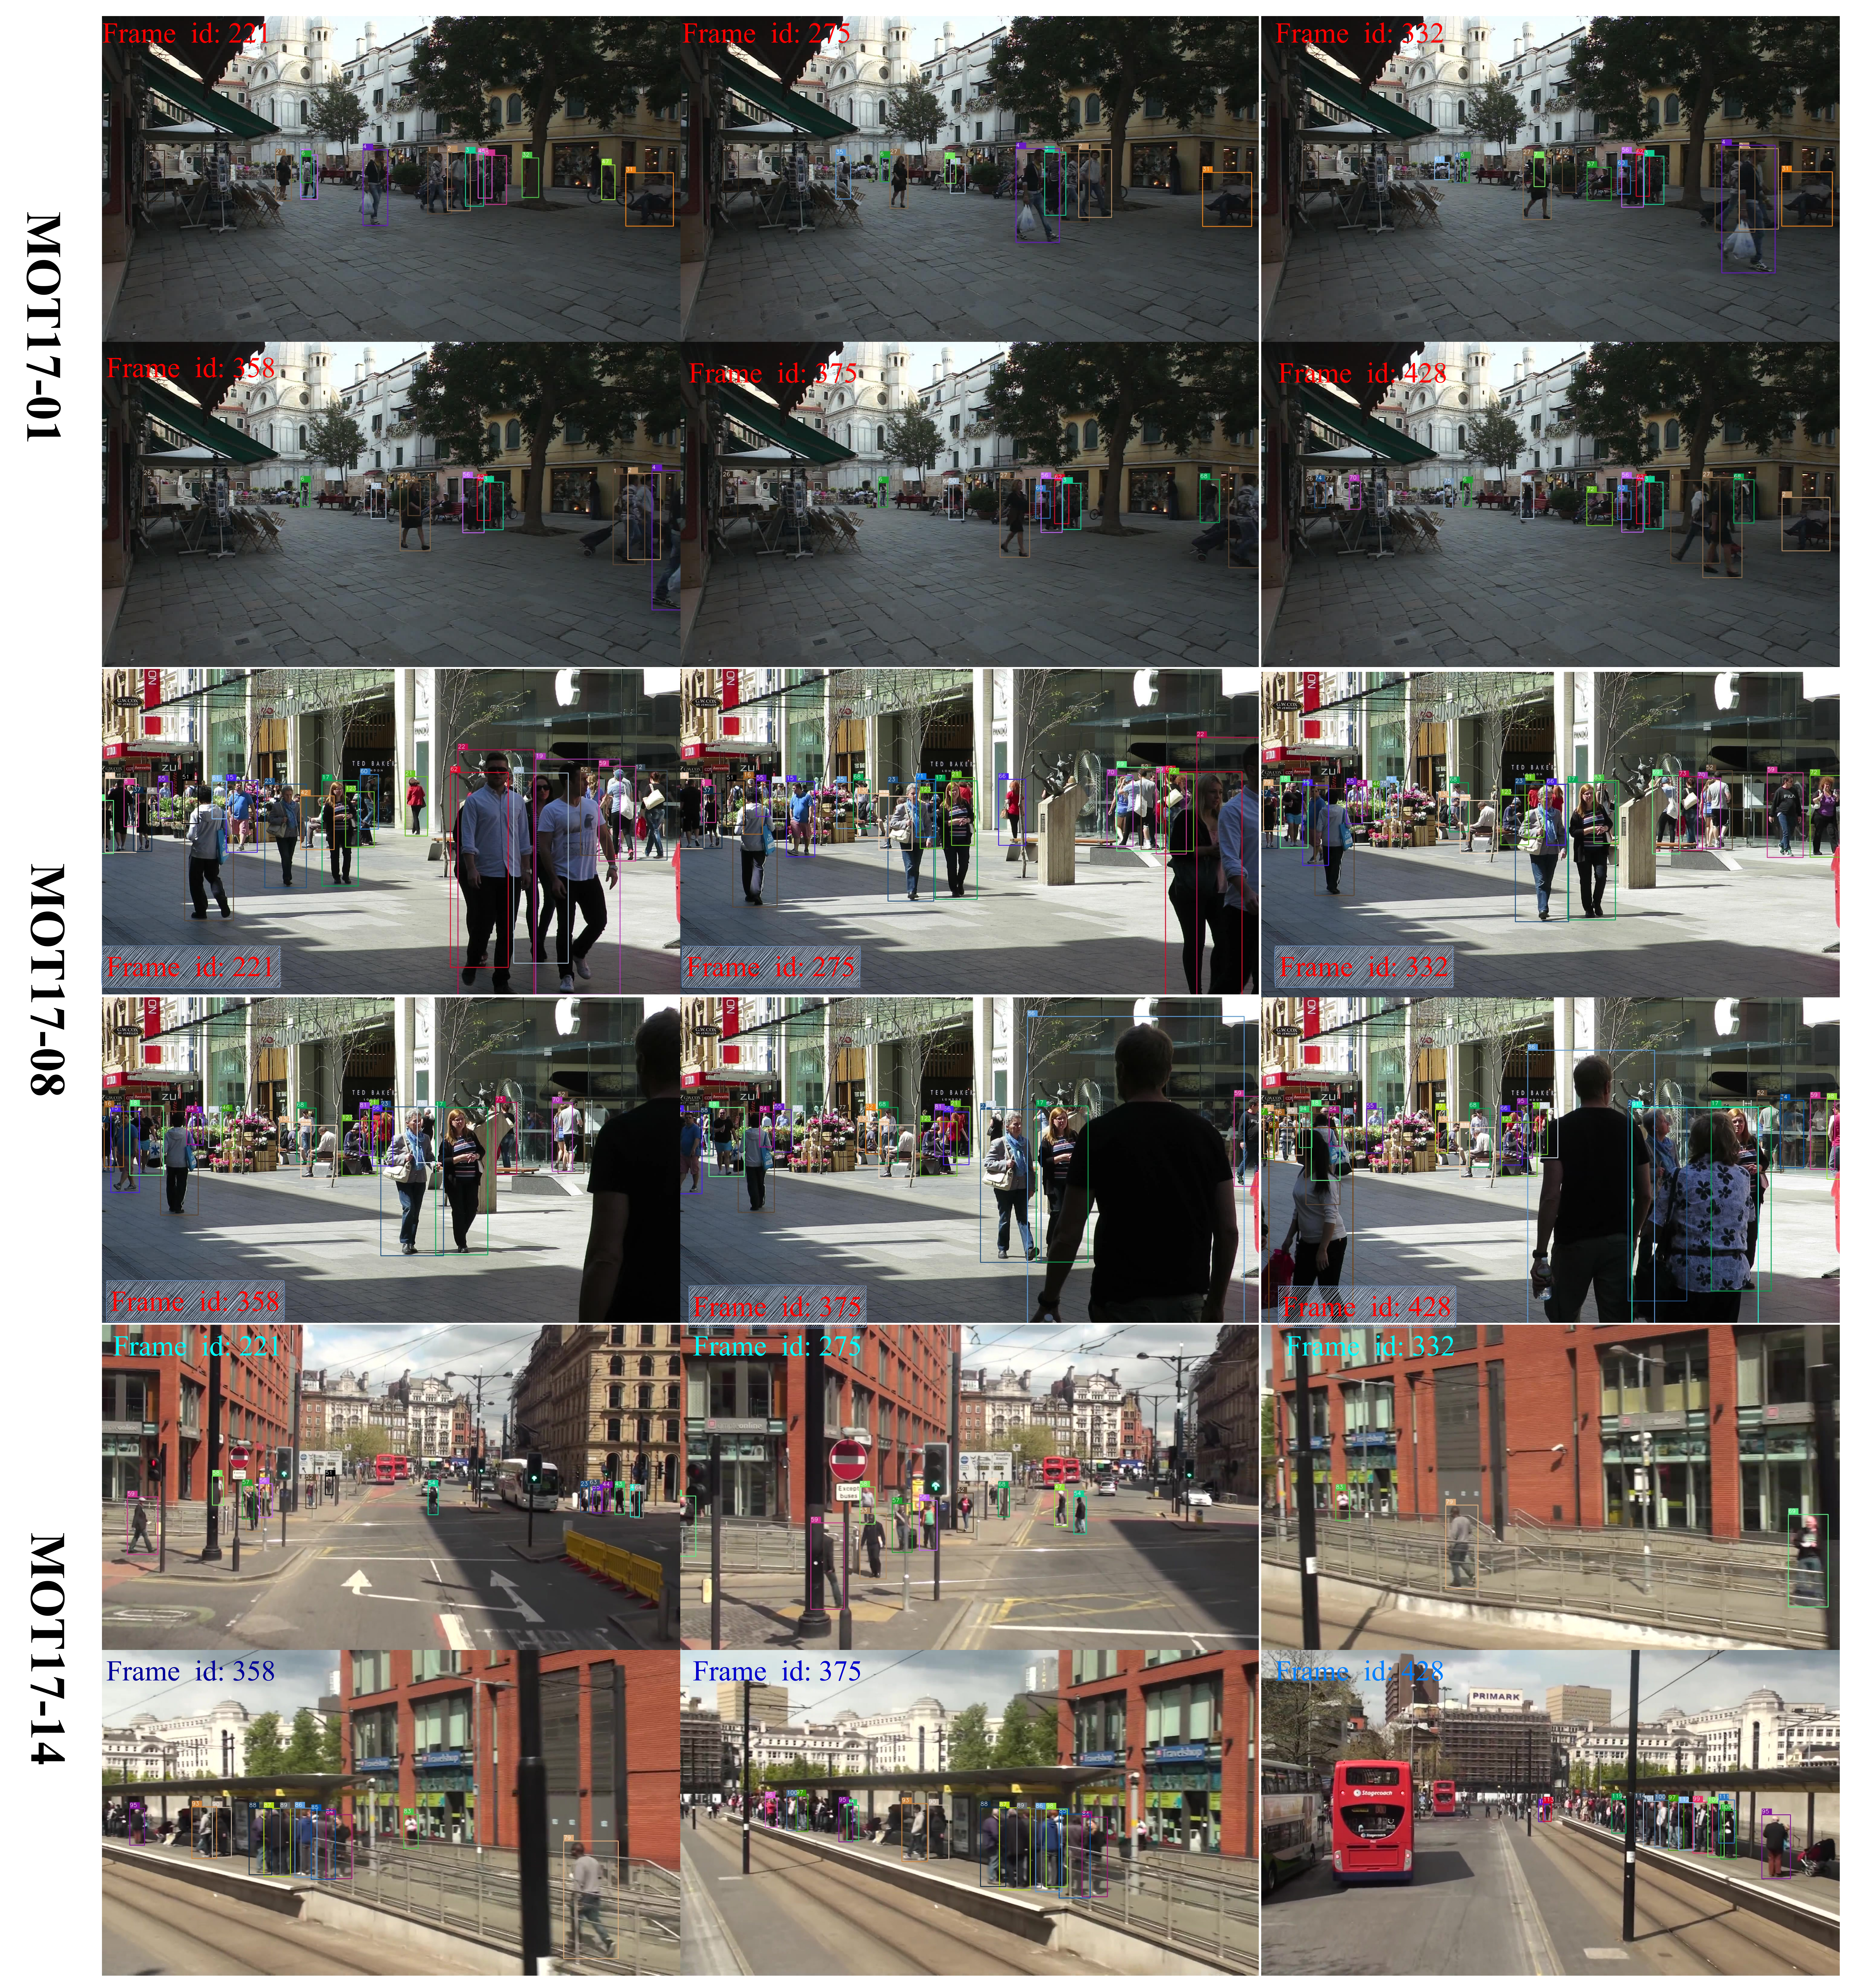}
	\end{center}
	\caption{Our model's visualization results on MOT17, where the same color represents the same object.}
	\label{vis_result_MOT17}
\end{figure*}

\begin{figure*}[t]
	\begin{center}
		\includegraphics[width=1\textwidth]{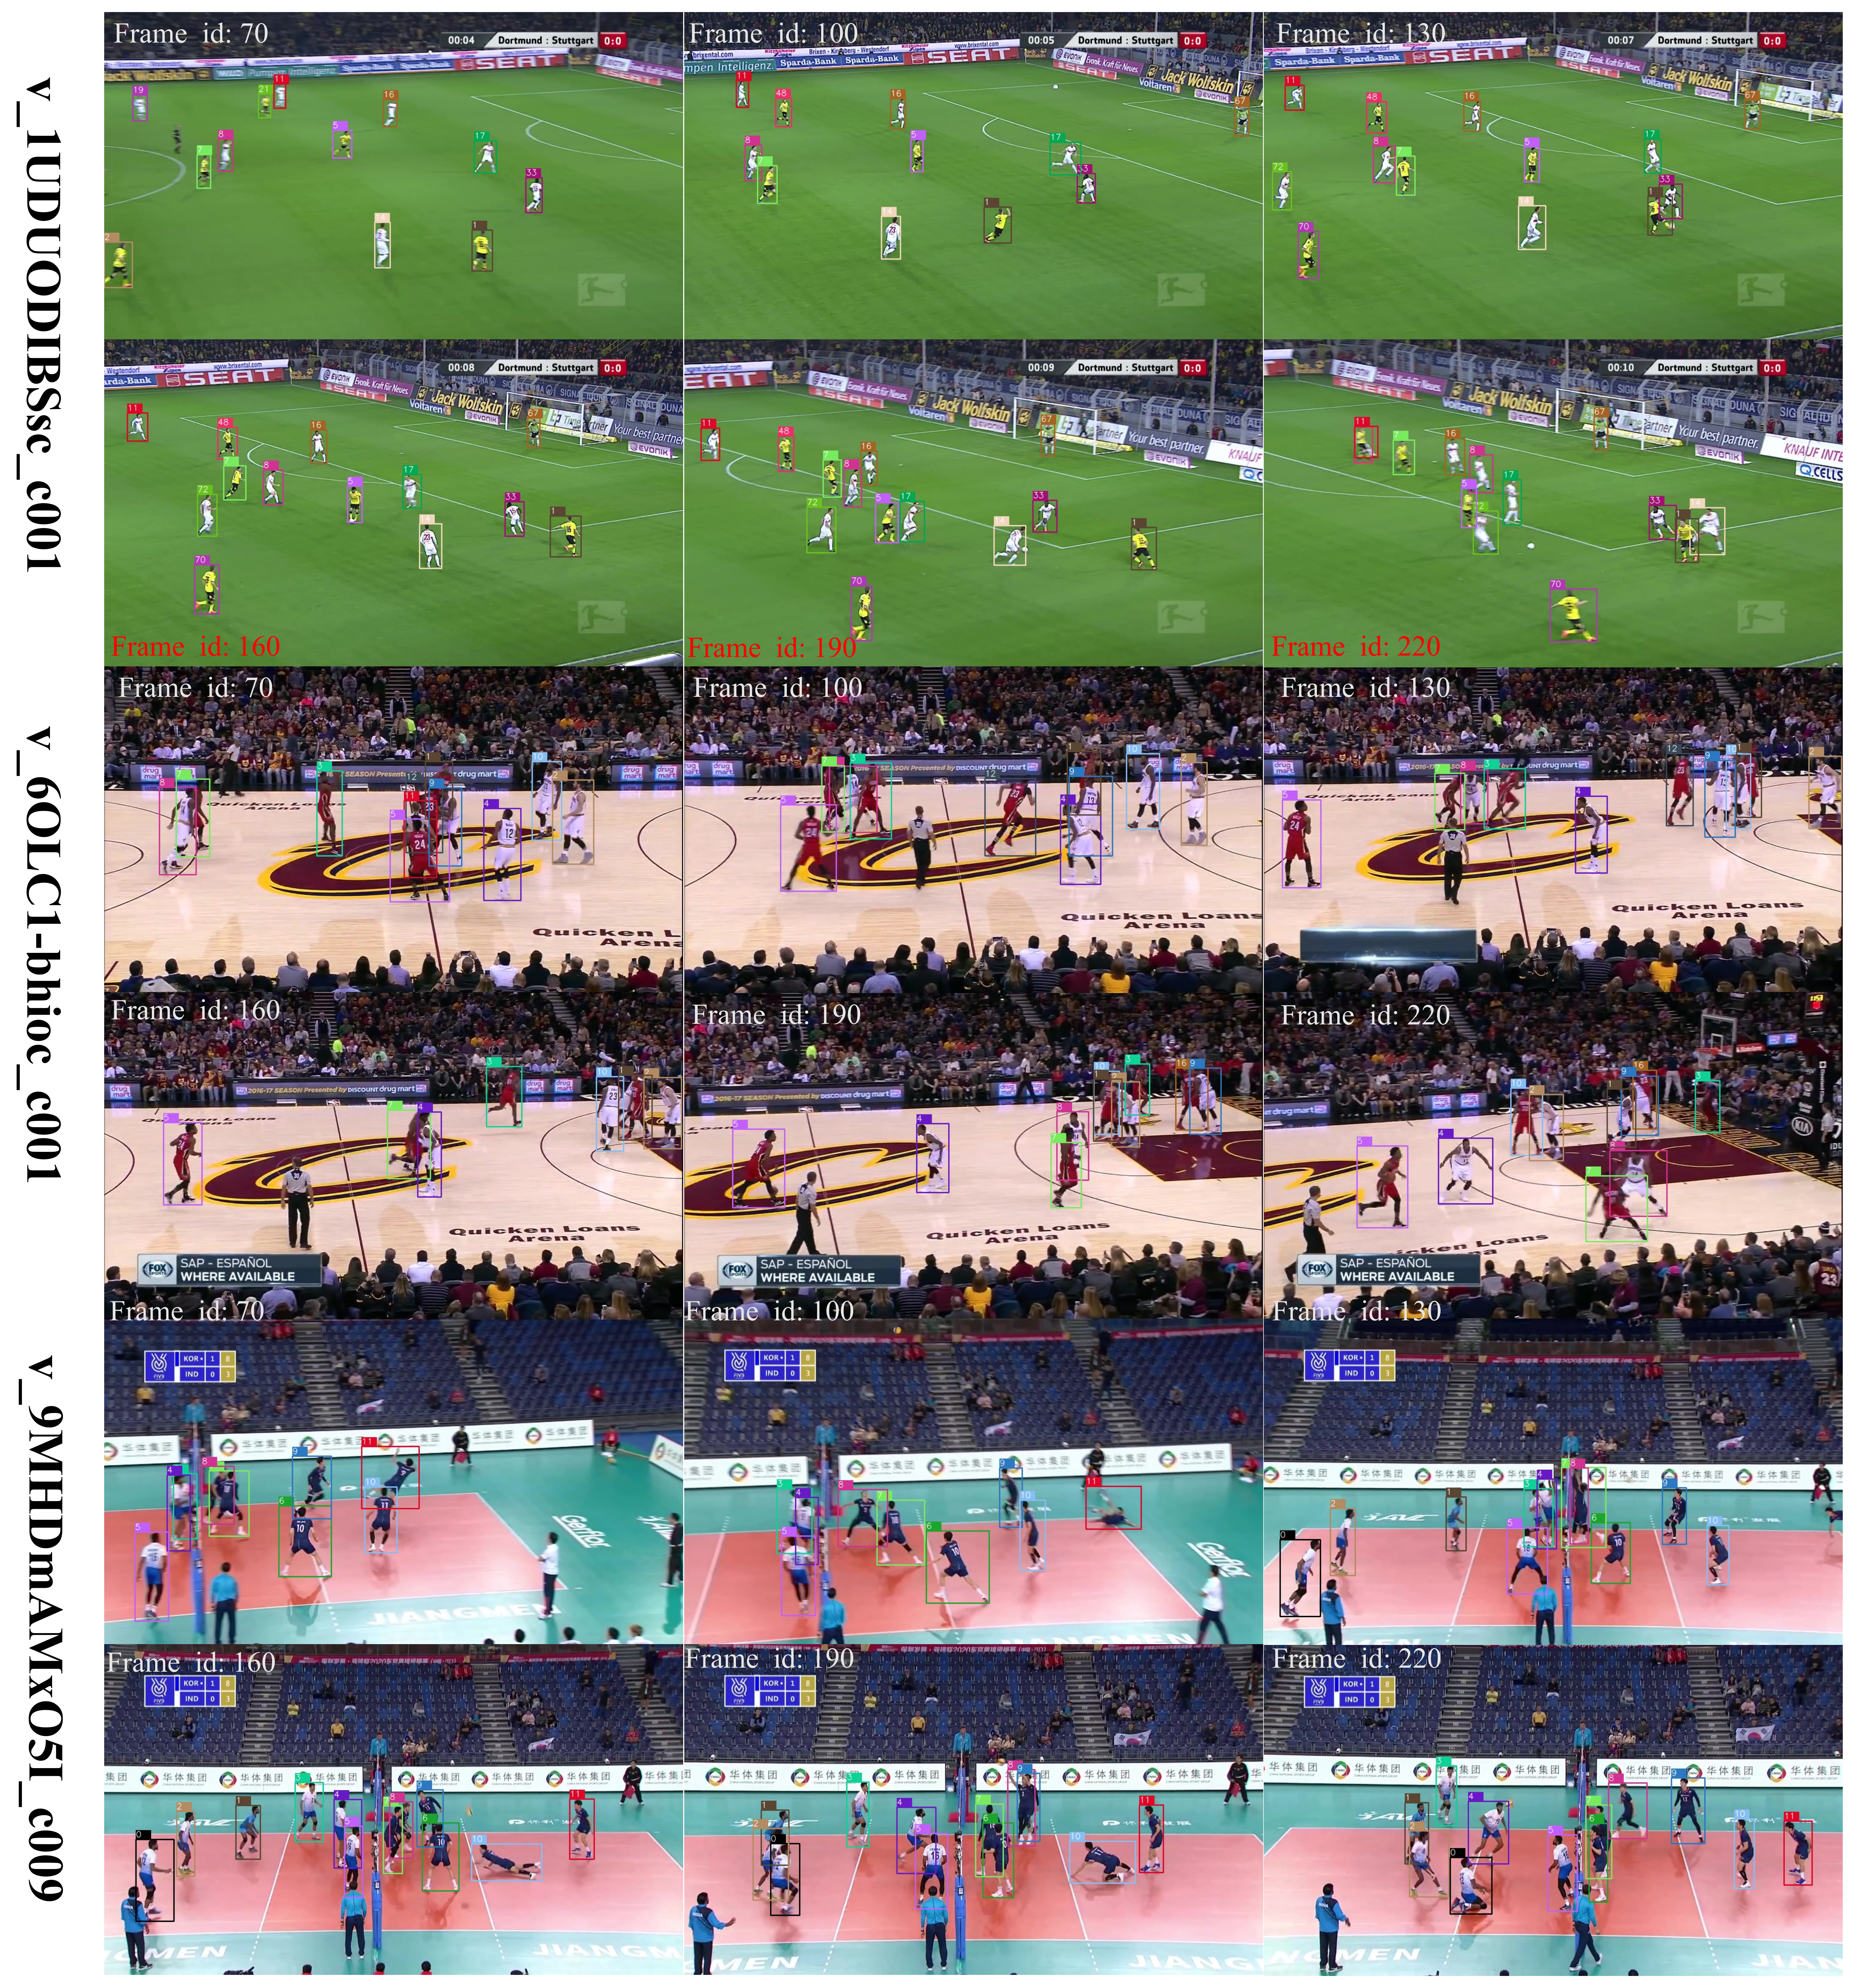}
	\end{center}
	\caption{Our model's visualization results on SportsMOT, where the same color represents the same object.}
	\label{vis_result_sportsmot}
\end{figure*}
